# Supplementary material for: MAG: Multi-Modal Aligned Autoregressive Co-Speech Gesture Generation without Vector Quantization
Source: arXiv:2503.14040 source file (2025-03-18)
Supplement: Supplementary file 1 [file 12-appendix.tex]

In the supplementary material, we provide a \textbf{supplementary video} to show:
\begin{itemize}
    \item The pipeline of the whole model as in the main paper.
    \item The comparison with baselines~(Sec.~\ref{supp:compare}).
    \item The effectiveness of each component in our framework~(Sec.~\ref{supp:ablation}).
    \item The applications of interpolating poses between different modalities~(Sec.~\ref{supp:app1}).
    \item The applications of semantic motion generation via new text prompt~(Sec.~\ref{supp:app2}).
\end{itemize}
We also give some explanations aligned with the video and list below.

\section{Comparisons with baselines}
\label{supp:compare}
We show the results comparing to all 
\section{Individual gestures from each generator}
\label{supp:ablation}
We present the generation results of our generators. 

\section{Ablation studies}
The use of MLPs is 

% \begin{figure}
%     \centering
%     \includegraphics[width=\linewidth ]{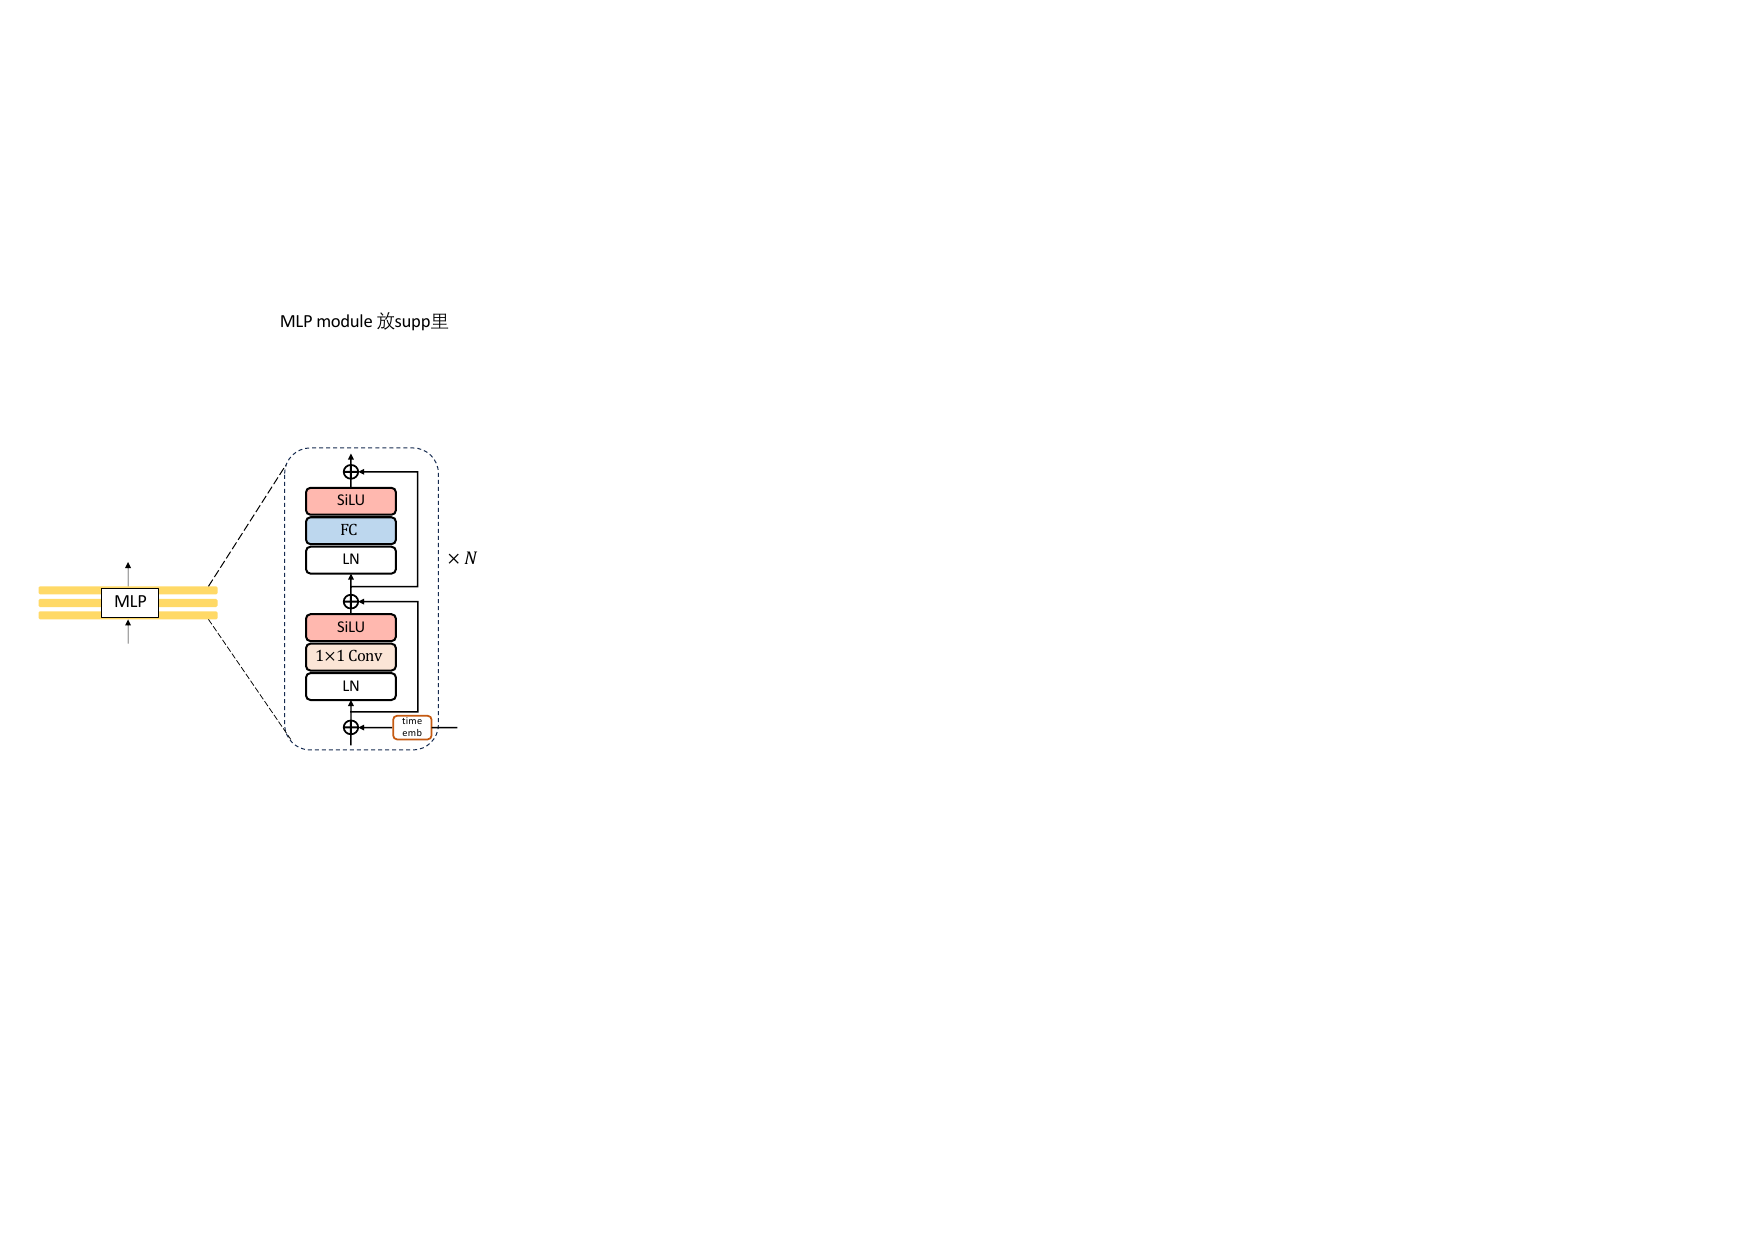}
%     \caption{Details of the MLP block.}
%     \label{fig:mlp_details}
% \end{figure}

\begin{table}[t]  
\centering
\begin{tabular}{cc|ccc}
\hline
        \# &  Act.  & FGD$\downarrow$ & BC $\uparrow$& Diversity$\uparrow$ \\ 
\hline
        4&SiLU   & 2.152 &   0.656  & 107.988   \\  \hline 
        4&ReLU   & 3.956  &  0.683 & 106.581   \\ 
        
        4&LReLU  & 5.847  & 0.682 & 105.668  \\ 
        
        4&LReLU$^\dag$   & 6.392  &  0.695 & 104.497  \\ \hline
        
        2&SiLU   & 8.243  &  0.689 & 106.115 \\ 
        
        6&SiLU   & 3.047 & 0.623 & 104.880    \\ 
        
        8&SiLU  & 4.184  & 0.655 & 104.876 \\ 
                \bottomrule

\end{tabular}
\caption{MLP architecture ablation. LReLU and LRELU$^\dag$ represent the LeakyRELU with the scope of 0.1 and 0.2, respectively. $\#$ represents the layer of MLP in the backbone.}
\label{table:MLP}
\end{table}
